# Supplementary material for: Overlapping subspaces and singular systems with application to Isogeometric Analysis
Source: arXiv:2408.17273 source file (2024-08-30)
Supplement: Supplementary file 1 [file appendix.tex]

% !TEX root = easy_adaptivity_and_solver_v7.tex

\section{Notes in infinite dimension}\label{App-1}

The abstract setting as described applies to finite dimensional spaces,
and the question about its applicability to the Hilbert and Banach
cases naturally arises.

First of all the sum of subspaces of an Hilbert space is not necessarily
closed.
This condition is contained in the assumption that \(V\) is an Hilbert
space and equation \eqref{eq:space}.

In the Hilbert setting, all subspaces are complemented, and in particular
they admit an orthogonal subspace.
This implies the existence of continuous and linear right inverses of \(S\).
The Hilbert structure is necessary also for Theorem~\ref{thm:S-inverse-norm}
where the right-inverse is not necessarily linear, but the construction
is based on trigonometric functions of the angles between the spaces.

Neither generalizes to Banach spaces: in each Banach that is not isomorphic
to an Hilbert space there exists a non-complemented 
subspace\cite{lindenstrauss1971complemented} and any surjective map admits
a continuous inverse if and only if its kernel is complemented.
The following example shows that even if the \(V_i\)-s are closed and
complemented, \(S\) could not have any continuos and linear right inverse.  

\begin{example}[\(S\) without continuous inverse in Banach] 
Let \(X\) be a Banach space that is not isomorphic to an Hilbert space
and \(Y\) be a closed uncomplemented subspace of \(X\). 
Take \(V:= Y\times X\), \(V_1= Y\times\{0\} \), \(V_2=\SPAN\{(v,v):v\in Y\}\).
Then the complement of both \(V_1\) and \(V_2\) is simply \(\{0\}\times Y\),
but \(V_1+V_2\) is not complemented.
\end{example}

As long as a continuous and linear right-inverse of \(S\) exists, it is
still possible to prove the spectral identity of 
Theorem~\ref{thm:preconditioner-spectrum}, but its application to the 
convergence of Krylov methods requires additional restrictions:
for instance Krylov methods cannot resolve infinite dimensional 
Jordan blocks.

\begin{proof}
To prove the first part it suffice to show that if
\(\lambda\not\in \spectrum(\wT)\) then \(\lambda\not\in \spectrum(T)\).
This is equivalent to show that if \((\wT -\lambda \wId)\) has
a continuous inverse \(\wJ_\lambda\) then it is possible to construct
an inverse of \( J_\lambda\) of \((T-\lambda \Id)\).
For any chosen right inverse \(S^{-1}_R\) of \(S\) we show that
\(S \wJ_\lambda S^{-1}_R \) is indeed the inverse of  \((T-\lambda \Id)\).

The key ideas are
\begin{itemize}
	\item \(\ker S\subseteq \ker \wT\)
	\item the split \(\wV=\ker S \oplus S^{-1}_R V\)
		given by the projectors \((\Id-S^{-1}_RS)\) and \(S^{-1}_RS\).
\end{itemize}
Together they imply \( \wT(\wId- S^{-1}_R S)=0\) because \(S(\wId- S^{-1}_R S)=0 \).

To see that \( J_\lambda\) is a right inverse use \eqref{eq:T-from-wT} 
and insert the above relations
\begin{align*}
	\anchor(T-\lambda \Id) S \wJ_\lambda S^{-1}_R = S (\wT -\lambda \wId)S^{-1}_R S\wJ_\lambda S^{-1}_R
	\\&=S (\wT -\lambda \wId) [ S^{-1}_R S +(\wId- S^{-1}_R S)]  \wJ_\lambda S^{-1}_R
	\\&= S (\wT -\lambda \wId)\wJ_\lambda S^{-1}_R=\Id.
\end{align*}
To see that \( J_\lambda\) is a left inverse we use additionally that
\(\wJ_\lambda|_{\ker S}=-\lambda^{-1}\wId\) in the form
\(\wJ_\lambda(S^{-1}_R S -\wId)=-\lambda^{-1}(S^{-1}_R S -\wId) \)
\begin{align*}
	\anchor S \wJ_\lambda S^{-1}_R (T-\lambda \Id)=S \wJ_\lambda S^{-1}_R S( \wT -\lambda \wId)S^{-1}_R,
	\\&= S \wJ_\lambda [ (S^{-1}_R S -\wId) + \wId ]( \wT -\lambda \wId)S^{-1}_R,
	\\&= \Id -S \lambda^{-1}(S^{-1}_R S -\wId) (\wT -\lambda \wId)S^{-1}_R =\Id.
\end{align*}

To construct an inverse of \((\wT-\lambda\wId)\) from the inverse
\(J_\lambda\) of \(T -\lambda \Id\) it is necessary to add
a correction that takes care of \(\ker S\).
In particular if \(\lambda\ne 0\), \(\range(T)\) is closed and 
\(B|_{\range(A)}\) is one-to-one
\[\wJ_\lambda := [ S^{-1}_R J_\lambda S -\lambda^{-1} (\wId-S^{-1}_RS)]\]
is the inverse of \((\wT-\lambda\wId)\).

This can be seen on each of the split \(\wV=\ker S \oplus S^{-1}_R V\)
separately.
On \(\ker S\) it acts both as a left 
\begin{align*}
	\anchor [ S^{-1}_R J_\lambda S -\lambda^{-1} (\wId-S^{-1}_RS)](\wT-\lambda\wId) (\wId-S^{-1}_RS)
	\\&=[ S^{-1}_R J_\lambda S -\lambda^{-1} (\wId-S^{-1}_RS)](-\lambda\wId)(\wId-S^{-1}_RS)
	\\& =[-\lambda^{-1} (\wId-S^{-1}_RS)](-\lambda\wId)(\wId-S^{-1}_RS)=(\wId-S^{-1}_RS),
\end{align*}
and a right inverse
\begin{align*}
	\anchor (\wT-\lambda\wId) [ S^{-1}_R J_\lambda S -\lambda^{-1} (\wId-S^{-1}_RS)] (\wId-S^{-1}_RS)
	\\&=(\wT-\lambda\wId) [-\lambda^{-1} (\wId-S^{-1}_RS)] (\wId-S^{-1}_RS)
	\\&=(-\lambda\wId)[-\lambda^{-1} (\wId-S^{-1}_RS)]=(\wId-S^{-1}_RS).
\end{align*}
On \(S^{-1}_R V\) it acts both as a left 
\begin{align*}
	\anchor [ S^{-1}_R J_\lambda S -\lambda^{-1} (\wId-S^{-1}_RS)](\wT-\lambda\wId) S^{-1}_RS
	\\&=[ S^{-1}_R J_\lambda S -\lambda^{-1} (\wId-S^{-1}_RS)] (S^{-1}_RTS -\lambda\wId) S^{-1}_RS
	\\&= [ S^{-1}_R J_\lambda S -\lambda^{-1} (\wId-S^{-1}_RS)] S^{-1}_R(T -\lambda\Id) S
	\\&=[ S^{-1}_R J_\lambda S] S^{-1}_R(TS -\lambda\Id) S= S^{-1}_RS,
\end{align*}
and a right inverse
\begin{align*}
	\anchor (\wT-\lambda\wId) [ S^{-1}_R J_\lambda S -\lambda^{-1} (\wId-S^{-1}_RS)]S^{-1}_RS= (S^{-1}_RTS -\lambda\wId)[ S^{-1}_R J_\lambda S]S^{-1}_RS
	\\&=S^{-1}_R(T -\lambda\Id)S[ S^{-1}_R J_\lambda S]S^{-1}_RS=S^{-1}_RS.
\end{align*}

\end{proof}
